# Supplementary material for: Active Learning with Partial Feedback
Source: arXiv:1802.07427 source file (2019-07-09)
Supplement: Supplementary file 1 [file appendix.tex]

\section{Experimental Results on CIFAR100}
We include additional results for CIFAR100 in Figure~\ref{fig:cifar100-top1}, \ref{fig:cifar100-labeling}, \ref{fig:cifar100-avgremain}, \ref{fig:cifar100-jumpstart}.

\section{Experimental Results on CIFAR10}
We include additional results for CIFAR10 in Figure~\ref{fig:cifar10-top1}, \ref{fig:cifar10-labeling}, \ref{fig:cifar10-avgremain}, \ref{fig:cifar10-jumpstart}.

\begin{figure}
  \centering
  {\small \textit{Model Performance} vs. \textit{Number of Binary Questions}}
  \includegraphics[width=\linewidth]{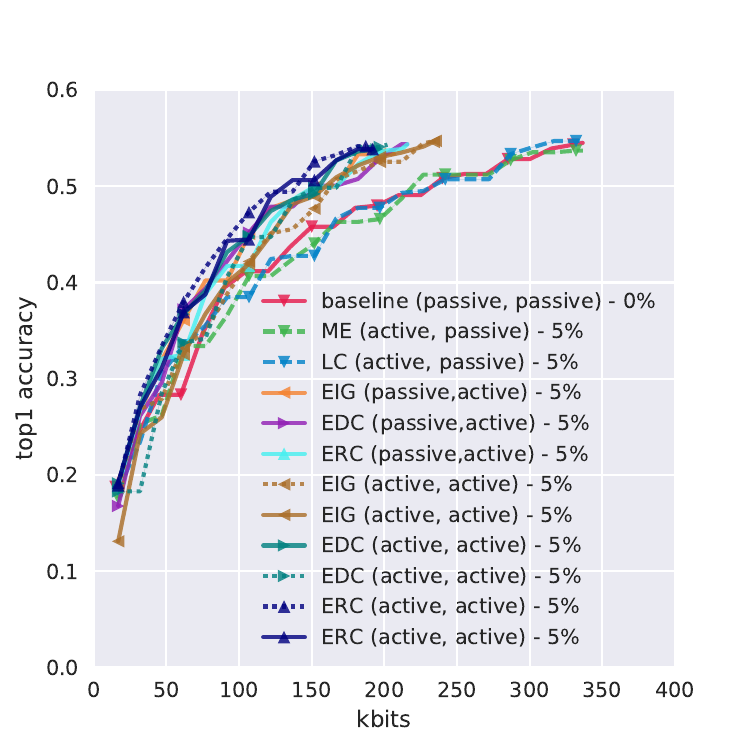}
  \caption{Model performance for CIFAR100}
  \label{fig:cifar100-top1}
\end{figure}

\begin{figure}
  \centering
  {\small \textit{Percentage of Full Labels} vs. \textit{Number of Binary Questions}}
  \includegraphics[width=\linewidth]{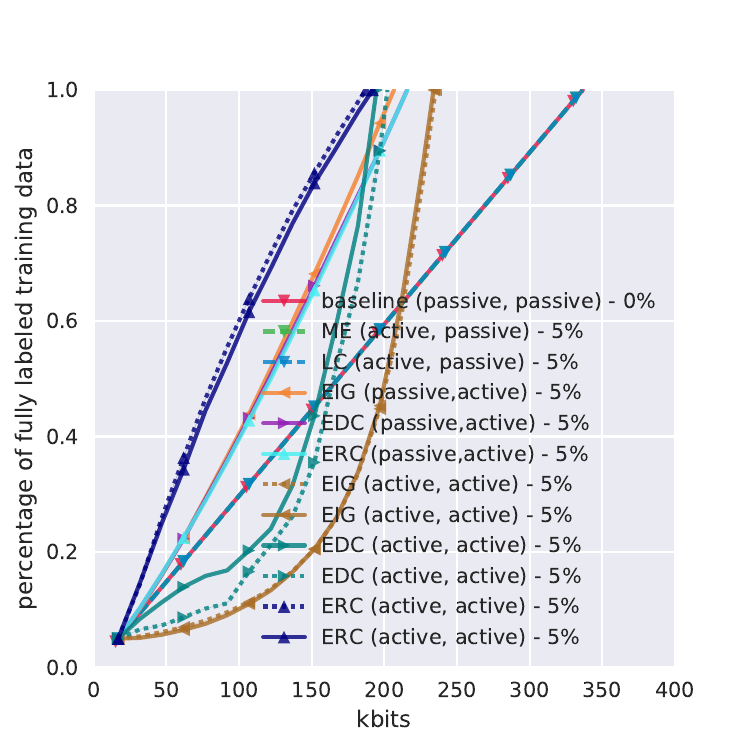}
  \caption{The percentage of fully labeled data for CIFAR100}
  \label{fig:cifar100-labeling}
\end{figure}

\begin{figure}
  \centering
  {\small \textit{Number of Remaining Classes} vs. \textit{Number of Binary Questions}}
  \includegraphics[width=\linewidth]{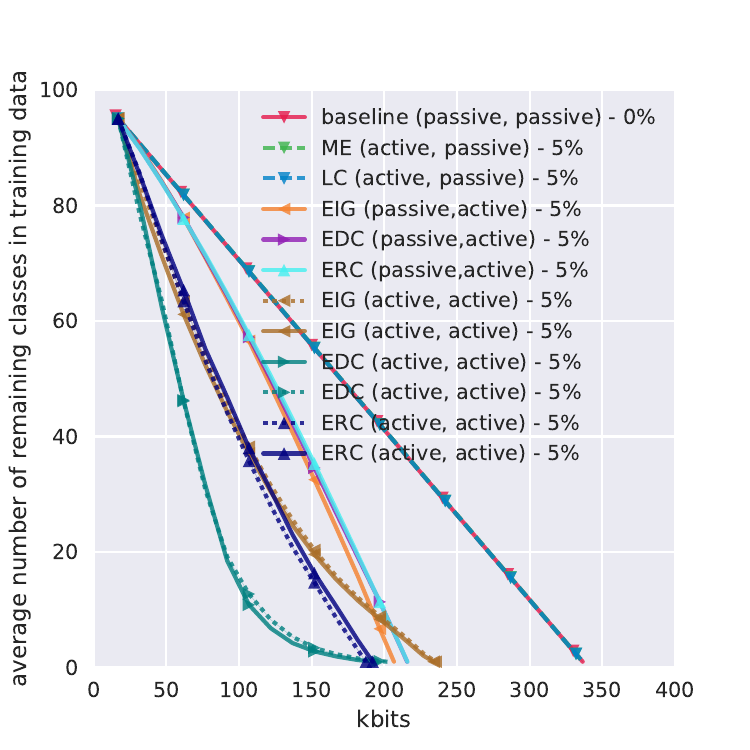}
  \caption{The number of remaining classes in the training set for CIFAR100}
  \label{fig:cifar100-avgremain}
\end{figure}

\begin{figure}
  \centering
  {\small \textit{Model Performance} vs. \textit{Number of Binary Questions}}
  \includegraphics[width=\linewidth]{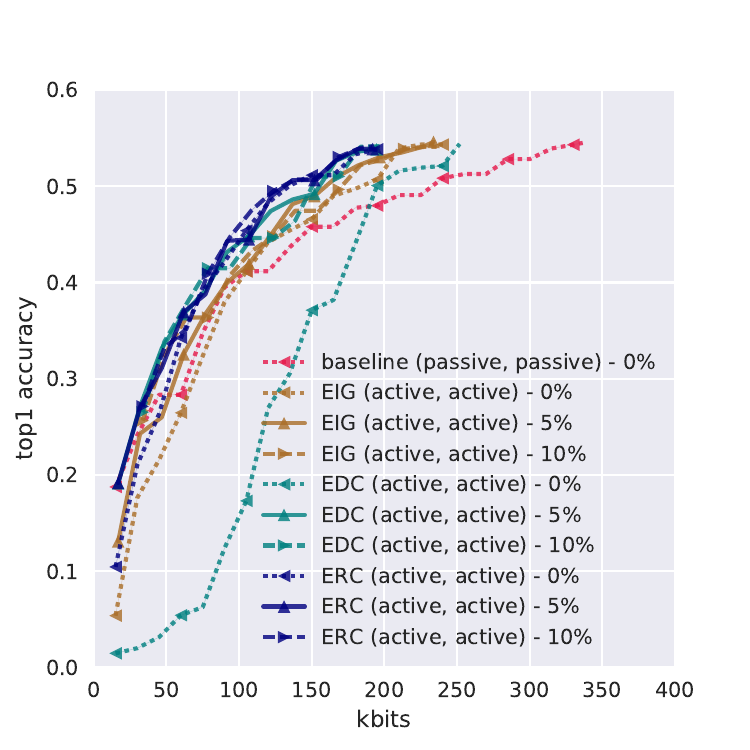}
  \caption{The effect of different amount of pre-labeled data for CIFAR100. }
  \label{fig:cifar100-jumpstart}
\end{figure}

\begin{figure}
  \centering
  {\small \textit{Model Performance} vs. \textit{Number of Binary Questions}}
  \includegraphics[width=\linewidth]{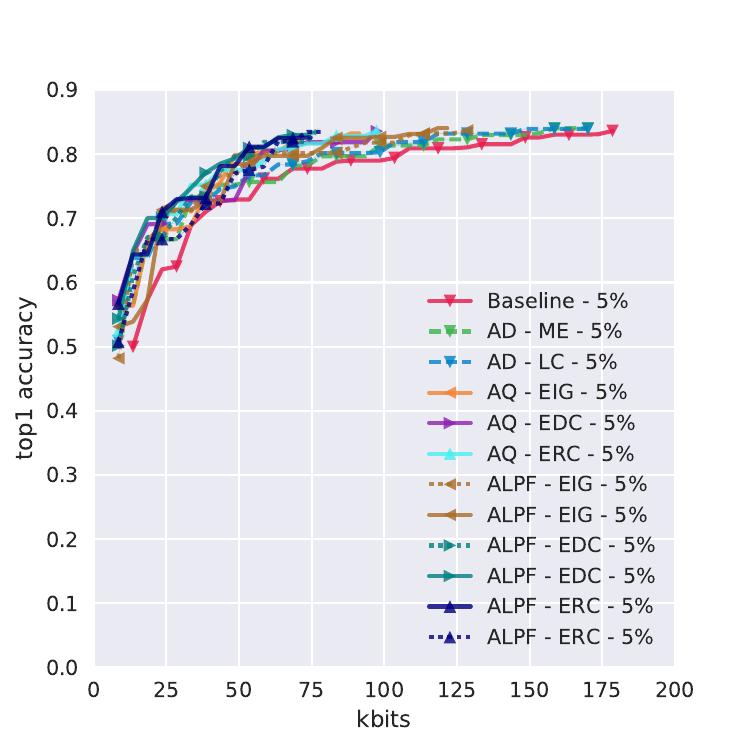}
  \caption{Model performance for CIFAR10}
  \label{fig:cifar10-top1}
\end{figure}

\begin{figure}
  \centering
  {\small \textit{Percentage of Full Labels} vs. \textit{Number of Binary Questions}}
  \includegraphics[width=\linewidth]{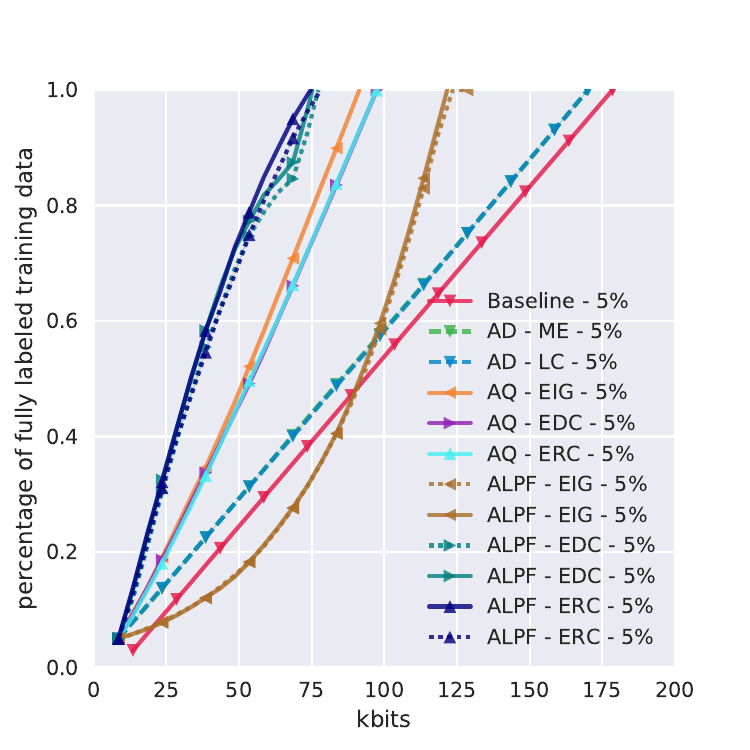}
  \caption{The percentage of fully labeled data for CIFAR10}
  \label{fig:cifar10-labeling}
\end{figure}

\begin{figure}
  \centering
  {\small \textit{Number of Remaining Classes} vs. \textit{Number of Binary Questions}}
  \includegraphics[width=\linewidth]{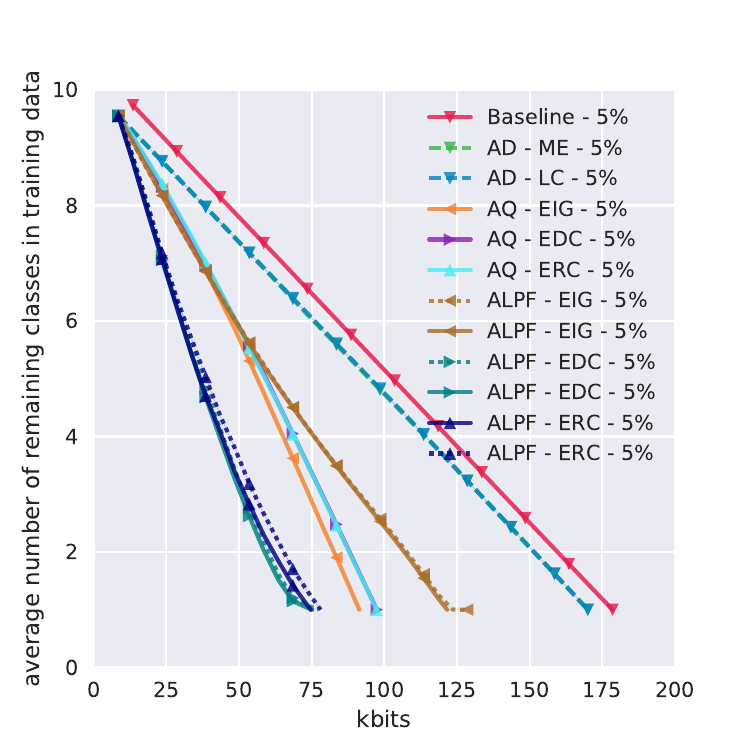}
  \caption{The number of remaining classes in the training set for CIFAR10}
  \label{fig:cifar10-avgremain}
\end{figure}

\begin{figure}
  \centering
  {\small \textit{Model Performance} vs. \textit{Number of Binary Questions}}
  \includegraphics[width=\linewidth]{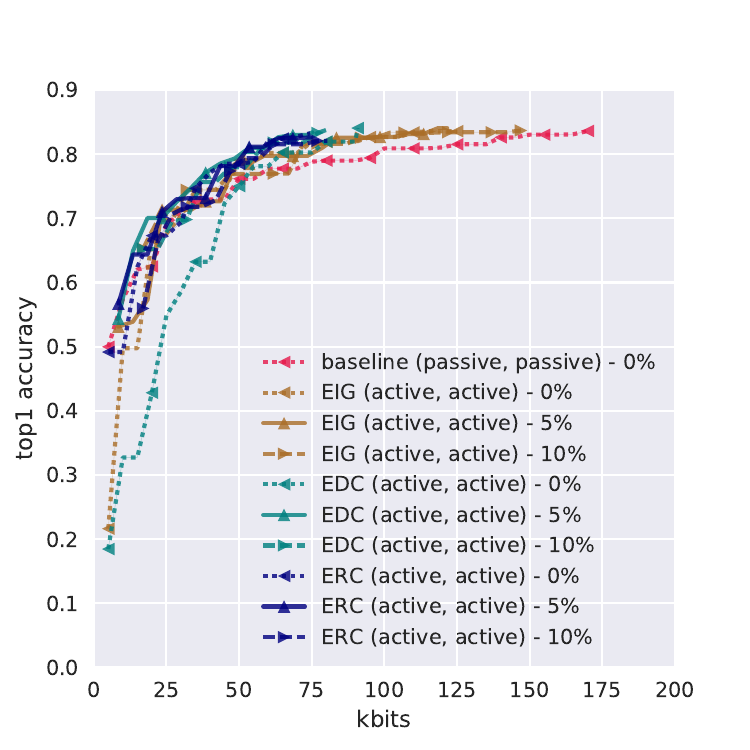}
  \caption{The effect of different amount of pre-labeled data for CIFAR10. }
  \label{fig:cifar10-jumpstart}
\end{figure}

%%% Local Variables:
%%% mode: latex
%%% TeX-master: "../main"
%%% End:
